# Supplementary material for: The Influence of Crosslinking and Deformation on Polymer Crystallization and Melting: A Molecular Dynamics Study
Source: arXiv:2601.11192 ancillary file (2026-01-16)
Supplement: Supplementary file 1 [file suppinfo.pdf]

# Supporting Information:

## The Influence of Crosslinking and Deformation on Polymer Crystallization and Melting: A Molecular Dynamics Study

Atmika Bhardwaj,<sup>†,‡,¶</sup> Huzaifa Shabbir,<sup>†,¶</sup> Jens-Uwe Sommer,<sup>\*,†,‡</sup> and Marco Werner<sup>\*,†</sup>

<sup>†</sup>*Theory of Polymers, Leibniz-Institut für Polymerforschung Dresden e.V., Hohe Strasse 6, 01069 Dresden, Germany.*

<sup>‡</sup>*Institute of Theoretical Physics, Technische Universität Dresden, Zellescher Weg 17, 01069 Dresden, Germany.*

<sup>¶</sup>*These authors contributed equally to this work.*

E-mail: sommer@ipfdd.de; werner-marco@ipfdd.de

### A Protocol steps

During NVT relaxation, samples with a higher magnitude of deformation start to crystallize if we let them relax for longer. Therefore, the relaxation time is chosen depending on the combination of network density and the magnitude of deformation in the system. In Figure S1(a), we observe the fluctuation in pressure values with straight lines drawn at the top-right indicating the mean converged pressure tensor components. For illustration purposes, we will use the specific case of *0bpc* and  $\lambda = 2.0$  in this as well as in the following protocol

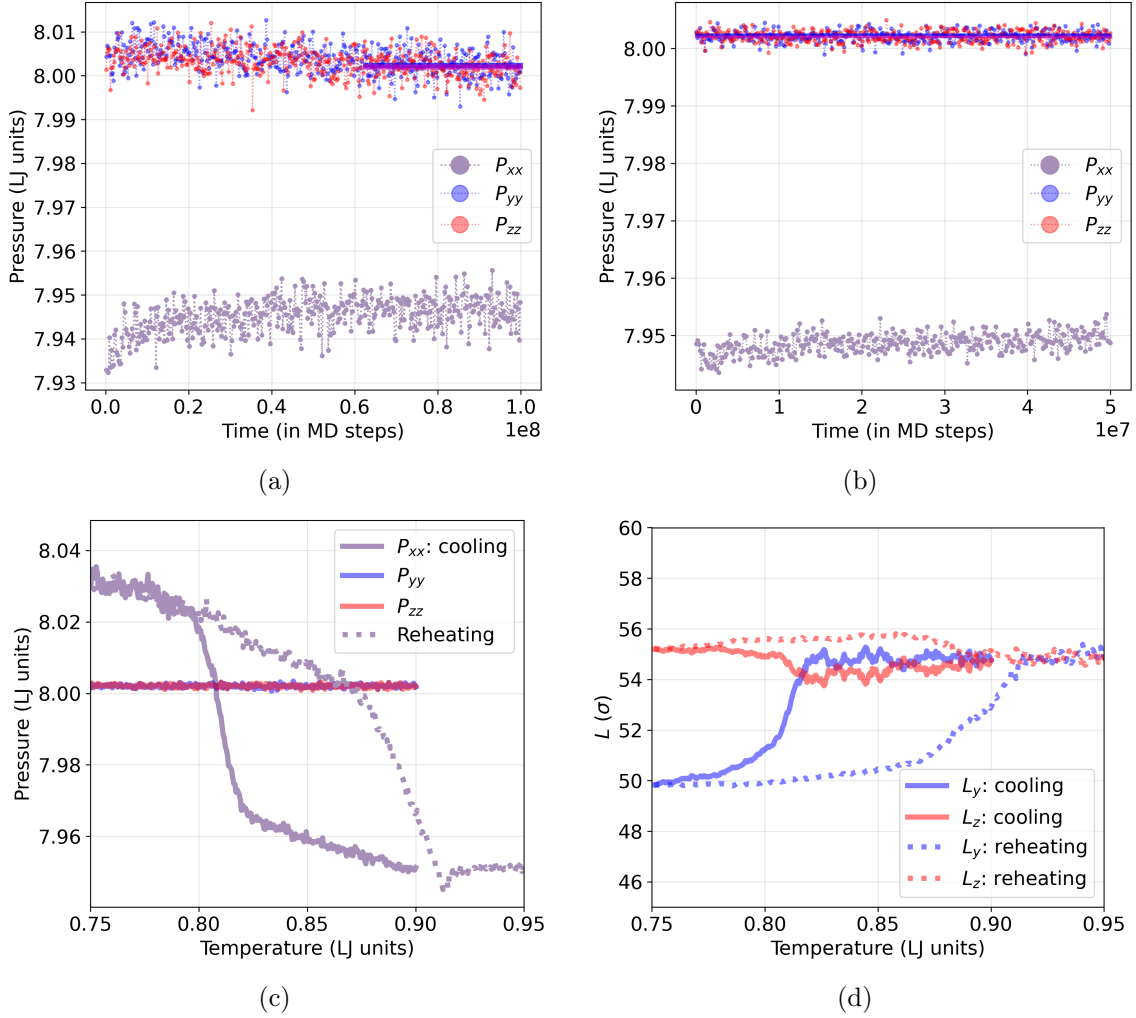

Figure S1: As discussed in Section 2, relaxation is performed in two stages of the protocol. For simplicity, we use the case of  $0bpc$  and  $\lambda = 2.0$  for illustrations. (a) NVT relaxation is performed in the fourth step of the protocol to extract the converged values of  $P_{yy}$  and  $P_{zz}$  as shown via two solid lines on the top right of the graph. (b) NPT relaxation as the fifth step of the protocol where pressure components  $P_{yy}$ ,  $P_{zz}$ , and the box length in the x-direction are fixed. (c, d) In the sixth and seventh steps of the protocol, we cool and reheat the system in NPT. (c) We see convergence in the values of  $P_{yy}$  and  $P_{zz}$  while  $P_{xx}$  shows a change in phase as temperature is varied. (d) The change in values of box length  $L$  in the y- ( $L_y$ ) and z- ( $L_z$ ) directions. The change in box length along the deformation axis  $L_x$  is not shown since it is maintained constant.

discussions.

The resulting pressure fluctuations from the fifth step of the protocol are shown in Figure S1(b), providing a detailed view of the component-wise pressure behavior during this relaxation process.

The evolution of the pressure component  $P_{xx}$  during the cooling and reheating cycles is shown in Figure S1(c). The other two pressure components ( $P_{yy}$  and  $P_{zz}$ ) are obtained from relaxation runs and remain fixed throughout these cycles. Figure S1(d) provides a visual representation of the change in the box dimensions in the y- and z-directions due to crystallization and melting. The box length in the x-direction ( $L_x$ ) is maintained at a fixed value throughout the simulation.

## B Comparisons with respect to $\lambda$

Figure S2 shows specific volume,  $v$  as a function of temperature,  $T$ , highlighting the effect of network density with constant  $\lambda$  in each plot. Starting from S2(a), we see the effect of crosslinks without any deformations in the system. From the heating cycles (discontinuous curves), it can be seen that the samples with higher network densities lose crystallinity and melt at lower temperatures as compared to *0bpc*.

The cooling cycles (continuous) with deformation contradicts this effect. As we increase both the network density and deformation, even the highly crosslinked network crystallizes early at higher temperatures. Furthermore, the systems show different densities both before and after crystallization. At higher temperatures, the presence of crosslinks slightly grows the density and the volume reduces slightly. But after crystallization, the crosslinks increase disturbance and frustration in the long-range order, and therefore, density goes down, and the  $v$  rises. For the case of  $\lambda = 3.0$  and *2bpc*,  $v$  overshoots after complete melting, indicating the deformation-induced pre-alignment in the system even before the cooling began.

Figure S3 highlights the evolution of stem lengths,  $d_{tt}$  with respect to network densities at the end of the cooling cycle. Uncrosslinked systems show longer  $d_{tt}$  as compared to the ones with crosslinks. Moreover,  $d_{tt}$  also increases with the total amount of deformation present in the system.

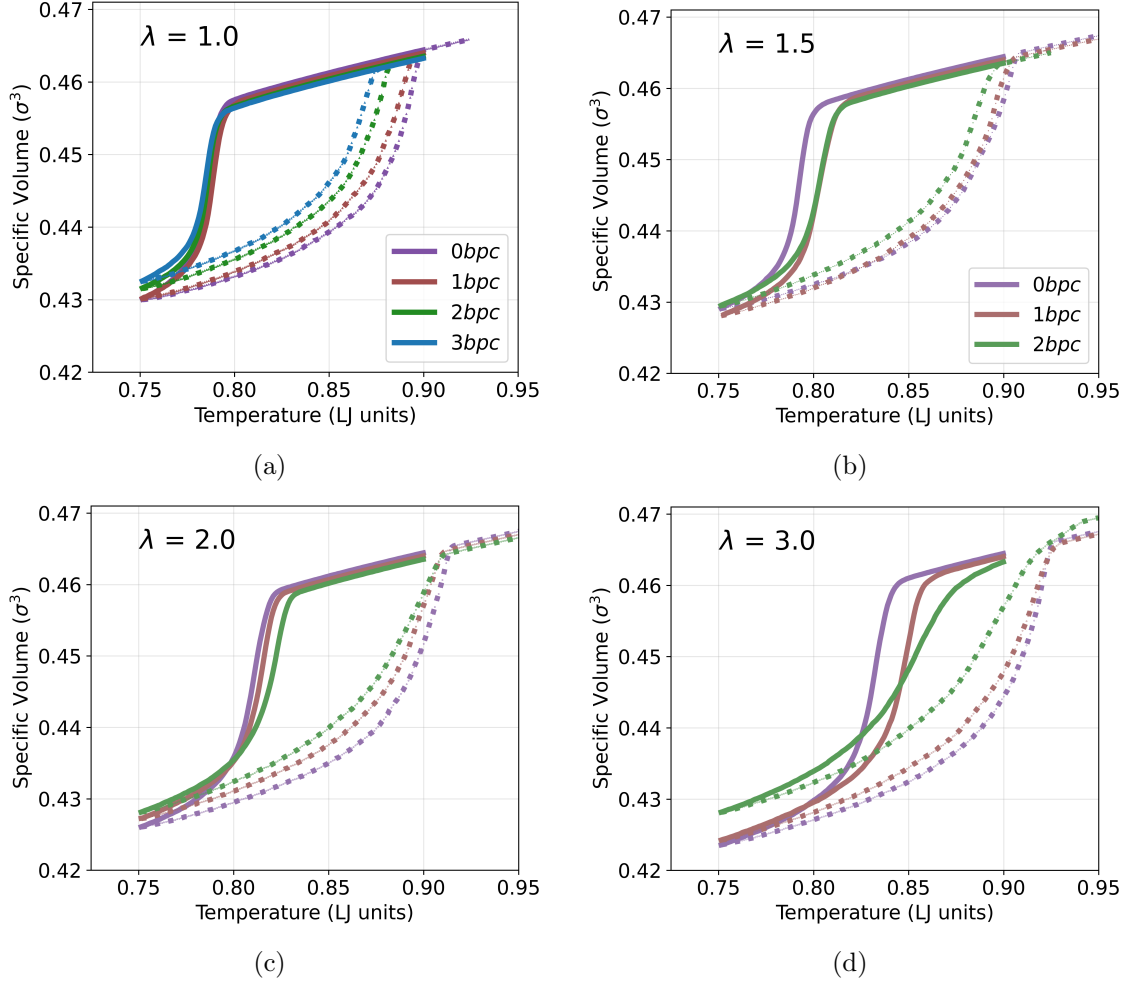

Figure S2: VT-phase diagrams for the cooling (continuous) and reheating (dotted) processes are shown with a fixed magnitude of deformation ratio  $\lambda$  in each plot. The network density or  $bpc$  varies in each case. Starting from the top-left  $\lambda$  is (a)1.0 or undeformed system, (b)1.5, (c)2.0 and, (d)3.0.

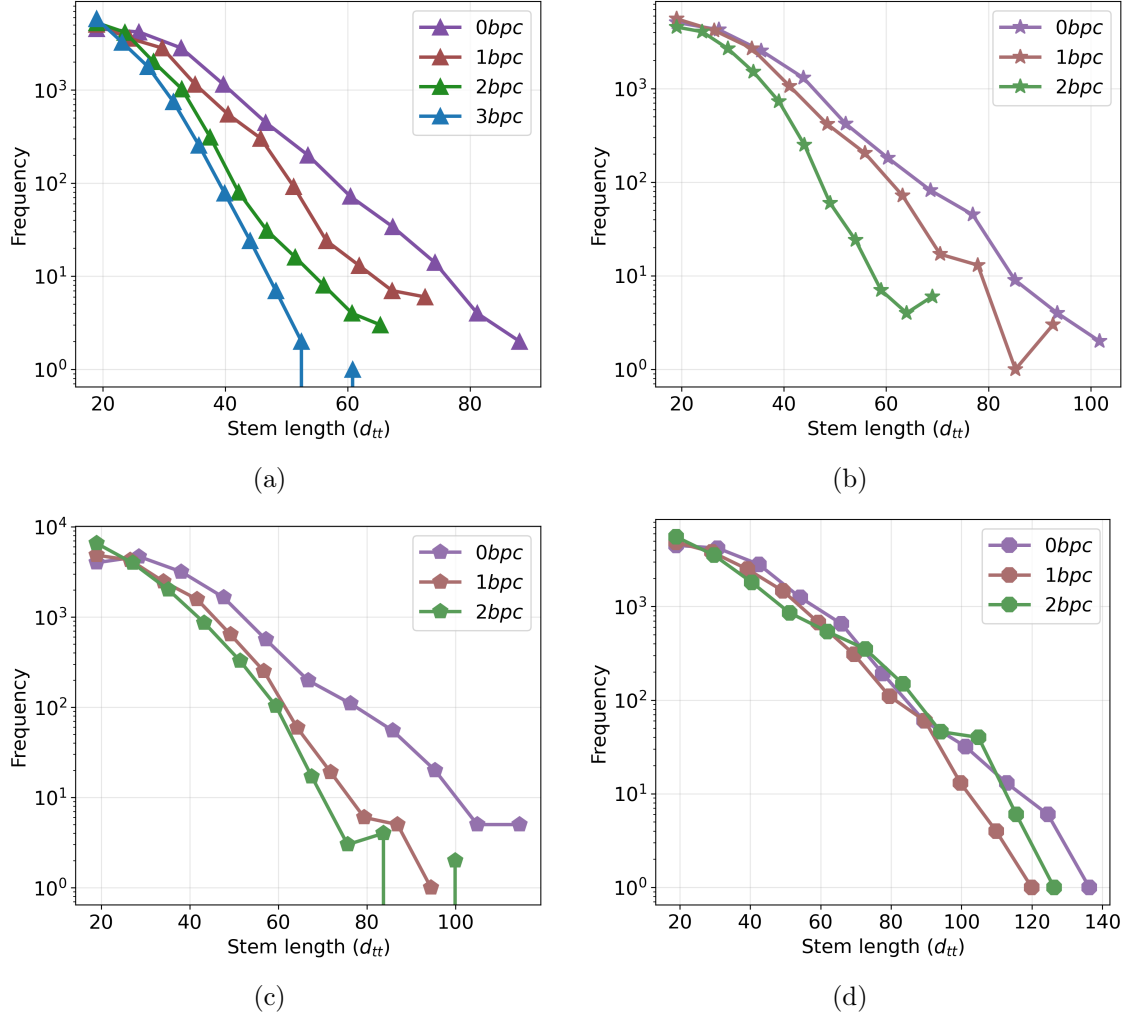

Figure S3: Stem length comparison between network densities (or *bpc*) while the deformation ratio  $\lambda$  is kept constant for each plot. Starting from the top-left  $\lambda$  is (a)1.0 or undeformed system, (b)1.5, (c)2.0 and, (d)3.0.
